# Supplementary material for: Approximately Counting and Sampling Hamiltonian Motifs in Sublinear Time
Source: arXiv:2503.09810 source file (2025-03-12)
Supplement: Supplementary file 1 [file cycles_appendix.tex]

\alg{
	{\bf \approxCountWithAdvice}$\;(n,\F, \eps, \delta, \onF)$ \label{alg:approx-count-with-advice}
	\smallskip
	\begin{enumerate}[itemsep=.2em]
            \item Let $\odelta=\min\{\delta/2,\eps/12\}$, and $\oeps=\eps/3$.
            \item Invoke \samplerPreprocess$(\onF, \oeps, \odelta)$ and let $\vec{V}$ be the returned values.  
            \item (Let $B$ denote the probability such that with probability $1-\odelta$, following the invocation of \samplerPreprocess$(\oeps,\odelta)$, every copy of $\F$ is returned with probability in $(1\pm\oeps)\frac{1}{B}$. )
             \item For $i=1$ to $t=\frac{B}{\onF}\cdot \frac{3\ln(4/\delta)}{(1-\oeps)\cdot \oeps^2}$ do: 
             \begin{enumerate}
                 \item Invoke \samplerAdvice$(n,\F, \vec{V})$
                 \item If a copy was returned,then set  $\chi_i=1$,  and otherwise set $\chi_i=0.$
             \end{enumerate}
             \item Set $\chi=\sum_{i=1}^t\chi_i$.
             \item Return $\hnF=\frac{B}{t}\cdot \chi$.
  \end{enumerate}
  }

\begin{theorem}[Basic Sampling implies approximate counting]
Let $G$ be a graph over $n$ vertices and $m$ edges, and let $\delta, \eps\in(0,1)$.
Further let $\onF$ be an estimate of $\countF$ and $\om$ an estimate of $m$.
Assume there exists a value $B=B(\onF,\om)$ and a pair of procedures as follows.
A preprocessing procedure \basicSamplerPreprocess$(n,\F, \onF, \om,\oeps,\odelta)$ 
that performs a preprocessing step and returns a set of variables $\vec{V}$,
and a sampling procedure \sampleAdvice{} as follows.
\begin{enumerate}
    \item If $\om \geq m$ and $\onF\geq \countF/4$ then 
    with probability at least $1-\delta$, following the invocation of \samplerPreprocess$(n,\F, \onF, \om, \oeps, \odelta)$, each invocation of  \sampleAdvice$(n,\F, \vec{V})$ independently samples a copy of $\F$ in $G$ such that each copy of $\F$ is returned with probability $(1\pm\eps)\cdot \frac{1}{B(\ov)}$.
    \iffalse
    \item If $\ov\leq  v/4$,  
    with probability at least $1-\delta$, following the invocation of \samplerPreprocess$(n,\F, \onF, \oeps, \odelta)$, each invocation of  \sampleAdvice$(n,\F, \vec{V})$ independently samples a copy of $\F$ in $G$ such that \emph{some, but maybe not all,} copies of $\F$ might be returned
    If a copy of $\F$ is returned, then it is returned  with probability $(1\pm\eps)\cdot \frac{1}{B(\ov)}$.
    \fi
     \item The query complexity and running time  of  \samplerPreprocess{} are $q_{p}$ and $t_{p}$, respectively.
     \item The query complexity and running time  of  \samplerPreprocess{} are  are $q_{s}$ and $t_{s}$, respectively.
\end{enumerate}
Then there exists a procedure \approxCountWithAdvice$(n,\F,\eps,\delta)$ as follows.
\begin{enumerate} 
    \item If $\onF\in [\countF/4,\countF]$, with probability at least $1-\delta$, \approxCountWithAdvice$(n,\F,\onF,\eps,\delta)$ returns a value $\hnF\in(1\pm\eps)\countF$.
    \item If $\onF>\countF$, then with probability at least $\eps/4$, \approxCountWithAdvice$(n,\F,\onF,\eps,\delta)$ returns a value $\hnF\leq(1\pm\eps)\countF$.
    \item  The query complexity of \approxCountWithAdvice{} is $O\left(q_p+\frac{B}{\onF}\cdot \frac{\ln(1/\delta)}{\eps^2}\cdot q_s\right)$.
    \item  The  running time of \approxCountWithAdvice{} is $O\left(t_p+\frac{B}{\onF}\cdot \frac{\ln(1/\delta)}{\eps^2}\cdot t_s\right)$.
\end{enumerate}
\end{theorem}
\begin{proof}
%talya HERE

By the setting of $\odelta$ and the premise on the preprocessing procedure, if $\om\geq m$ and $\onF\geq \countF$, then with probability at least $1-\odelta=1-\min\{\delta/2,\eps/12\}$, 

We say that the invocation of \samplerPreprocess$(n,F,\onF, \om, \oeps, \odelta)$ is successful if following it, 
each  invocation of \samplerAdvice$(n,F,\onF, \om, \vecV)$ independently samples a copy of $\F$ such that each copy is returned with probability in $(1\pm\oeps)\frac{1}{B}$. We denote this event by $E_{sp}$ (where $sp$ stands for a successful preprocessing step).

We first consider the case that $\onF>\countF$.
Conditioned on $E_{sp}$, for every $i$, $\EX[\chi_i]\leq(1+\oeps)\frac{\countF}{B}=(1+\eps/3)\frac{\countF}{B}$.
Hence, $\Ex[\chi]\leq (1+\eps/3) \cdot t\cdot \frac{\countF}{B}$.

By Markov's inequality, for $\eps<1$,
\begin{align}\label{eq:markov_gen}
\Pr\left[\chi>(1+\eps/2)\cdot \EX[\chi]\right]<\frac{1}{1+\eps/2}<1-\eps/3\;.
\end{align}
Denote by $E_{mar}$ the event that $\chi\leq (1+\eps/2)\EX[\chi]$.
By the first premise in the theorem, the setting of $\odelta=\min\{\delta/2, \eps/12\}$,  and by Equation~\eqref{eq:markov_gen}, 
$\Pr[\overline{E}_{sp}]+\Pr[\overline{E}_{mar}\mid E_{sp}]\leq \eps/12 + 1-\eps/3=1-\eps/4$.
 Therefore, with probability at least $\eps/4$, both $E_{sp}$ and $E_{mar}$ occur\talya{?}, and so
 $\chi<(1+\eps/2)(1+\eps/3)\cdot t\cdot \frac{\countF}{B}\leq (1+\eps) \cdot t\cdot \frac{\countF}{B}.$ 
By the setting of $\hnF=\frac{B}{t}\cdot \chi$, 
with probability at least $1-\eps/4$,
$\hnF<(1+\eps)\countF$, and the second item in the theorem holds.

We now consider the case that  $\onF\in [\countF/4,\countF]$.

Conditioned on $E_{sp1}$, for every $i$, $\EX[\chi_i]\in (1\pm\oeps)\frac{\countF}{B}$.
Since the $\chi_i$'s are $\{0,1\}$ independent random variables,
  then by the multiplicative Chernoff's bound and by the setting of $t$ in Step~\ref{step:for-loop}, for the case that $\onF\geq \countF/4$,
\begin{align}\label{eq:chernoff_gen}
\Pr\Big[\left|\chi-\Ex[\chi]\right|>\oeps\cdot \Ex[\chi]\Big]\leq 2\exp\left(-\frac{\oeps^2\cdot \Ex[\chi]}{3}\right)\leq 2\exp\left(-\frac{\oeps^2\cdot (1-\oeps)\cdot \frac{B}{\onF}\cdot \frac{3\ln(2/\delta)}{(1-\oeps)\cdot\oeps^2}\cdot \frac{\countF}{B}}{3}\right)\leq \frac{\delta}{2}\;.
\end{align}

Denote by $E_{ga}$ the event that $\chi\in(1\pm\oeps)\EX[\chi]$. 
Conditioned on the event $E_{sp1}$ (defined earlier in the proof), $\Ex[\chi]\in (1\pm\oeps)\cdot t\cdot \frac{\countF}{B}$,
and conditioned on $E_{ga},$ $\chi \in (1\pm\oeps)\EX[\chi]$. Also, $\hnF=\frac{B}{t}\cdot \chi$. Hence, conditioned on $E_{sp1}$ and $E_{ga}$,
$$\hnF\in (1\pm\oeps)^{2}\cdot \countF\in(1\pm\eps)\cdot \countF,$$ 
where the last inequality is by the setting of $\oeps=\eps/3$. 
By the first premise in the theorem,  and by Equation~\eqref{eq:chernoff_gen}, $\Pr[\overline{E}_{sp1}] + \Pr[\overline{E}_{ga}\;|\; E_{sp1}] \leq 
\min\{\delta/2,\eps/12\}+\delta/2\leq \delta$. 
Therefore, we get that with probability at least $1-\delta$, $\hnF\in(1\pm\eps)\cdot\countF$, 
  and  the first item in the theorem holds.

%%%%%%%%%%%%%%%%%%%%%%%%%%%%%%%%%%%%%%%%%%
%second promise

The query complexity of the algorithm is $O\left(q_{sp}+\frac{B}{\onF}\cdot q_{s}\right)$, and the running time is $O\left(t_{sp}+\frac{B}{\onF}\cdot t_{s}\right)$.

\end{proof}
